# Supplementary material for: ChronicleRec: Pre-training Temporally Anchored Tokens for Lifelong User Modeling
Source: arXiv:2609.12375 source file (2026-09-11)
Supplement: Supplementary file 1 [file 6.appendix.tex]

\section{Appendix}


As summarized in Table~\ref{tab:fm_representation_taxonomy}, existing
pretrained or shared-upstream recommendation models expose their learned
knowledge through substantially different representation interfaces.
Early approaches typically compress user history into a single global
embedding, while subsequent methods retain multiple global, aspect-specific,
or scope-specific representations. More recent sequential foundation models,
such as VISTA and LLaTTE, further introduce multiple latent or query tokens
to summarize the behavior sequence. However, these summary slots do not
explicitly correspond to distinct positions along the user's behavioral
timeline. In contrast, ChronicleRec represents the user as a compact
\emph{temporal-token memory}, where each Chronicle Token is anchored to a
specific temporal position and summarizes a causally bounded historical
prefix.

\begin{table*}[t]
\centering
\caption{
Comparison of representation interfaces in pretrained or shared-upstream
recommendation models.
``TI'' denotes target-independent representations that can be reused across
candidate scoring.
}
\label{tab:representation_interface}
\scriptsize
\setlength{\tabcolsep}{3pt}
\renewcommand{\arraystretch}{1.12}

\begin{tabularx}{\textwidth}{
@{}
p{1.75cm}
p{2.20cm}
p{2.40cm}
p{1.30cm}
p{3.00cm}
X
p{1.45cm}
@{}
}
\toprule

\textbf{Method} &
\textbf{Upstream Paradigm} &
\textbf{Downstream Representation} &
\textbf{\# Reps.} &
\textbf{Extraction / Layout} &
\textbf{Temporal Semantics \& Information Flow} &
\textbf{TI?}
\\

\midrule

Amazon GenPretrain~\cite{chitlangia2023scaling}
&
Self-supervised sequential pretraining
&
User / sequence embedding
&
1
&
Final hidden state at the last timestep
&
One global representation of the preceding sequence; history is modeled
autoregressively and causally.
&
Yes
\\

\addlinespace[2pt]

CLUE~\cite{shin2023clue}
&
General-purpose pretrained user encoder
&
Service-specific user embedding
&
1 / service
&
Mean pooling over Service Transformer states
&
Each representation corresponds to a service rather than a temporal position;
no multi-token temporal structure.
&
Yes
\\

\addlinespace[2pt]

Snap GPUM~\cite{fang2024gpum}
&
General-purpose self-supervised behavioral model
&
User embedding
&
1
&
Pooling over behavior-level hidden states
&
The entire behavioral sequence is compressed into one global user
representation.
&
Yes
\\

\addlinespace[2pt]

Snap UUM~\cite{ju2025uum}
&
Foundational cross-domain user model
&
Long-term user embedding
&
1
&
Cross-domain sequential modeling followed by a final user representation
&
One global cross-domain representation; internal bottleneck tokens are not
exported as user-memory tokens.
&
Yes
\\

\addlinespace[2pt]

Meta SUM~\cite{zhang2024sum}
&
Shared upstream user model
&
User embeddings
&
Fixed $K$; $K{=}2$ in production
&
User tower compresses large-scale user-side features into a few output
embeddings
&
Multiple learned global representations, but with no explicit chronological
ordering or temporal-slot semantics.
&
Yes
\\

\addlinespace[2pt]

LFM4Ads~\cite{zhang2025lfm4ads}
&
Pretrained advertising foundation model
&
$\mathrm{UR}(u)$, $\mathrm{IR}(i)$,
$\mathrm{CR}(u)$, $\mathrm{CR}(i)$
&
Few fixed types
&
User, item, and cross towers; sample-level cross representations are further
aggregated
&
Different representations encode \emph{representation scope}
(user, item, or user--item interaction), rather than different temporal
positions.
&
Mostly
\\

\addlinespace[2pt]

VISTA~\cite{chen2026vista}
&
Foundational upstream sequence summarization
&
User summary embeddings
&
Fixed $K$
&
Learnable virtual-seed bank summarizes the complete user interaction history
&
Summary slots have learned latent identities but no explicit temporal anchors;
each summarizes the global history rather than a distinct historical prefix.
&
Yes
\\

\addlinespace[2pt]

LLaTTE~\cite{xiong2026llatte}
&
Large asynchronous upstream sequential model
&
One/few fixed-size sequence summaries
&
$n_q \!\rightarrow\!$ few
&
Learnable queries $q_{1:n_q}$ are appended \emph{after} the complete behavior
sequence; query states are subsequently projected
&
Queries are causally ordered, but every query is placed after $H_{1:T}$ and
can therefore access the complete behavioral horizon; no distinct temporal
cutoffs.
&
Yes
\\

\addlinespace[2pt]

\textbf{ChronicleRec (Ours)}
&
\textbf{Pretrained sequential representation model}
&
\textbf{Chronicle Token sequence}
&
\textbf{Fixed $P$}
&
\textbf{Learnable queries are interleaved at explicit temporal anchor positions}
&
\textbf{Chronologically ordered and causal: each token has a distinct receptive
field $\mathcal{R}(\mathbf{c}_k)=H_{\leq a_k}$, with
$a_1<\cdots<a_P$.}
&
\textbf{Yes}
\\

\bottomrule
\end{tabularx}
\end{table*}
